# Supplementary material for: The interplay of local electron correlations and ultrafast spin dynamics in fcc Ni
Source: arXiv:2210.13162 ancillary file (2022-10-24)
Supplement: Supplementary file 1 [file Lojewski_supplement.pdf]

# The interplay of local electron correlations and ultrafast spin dynamics in fcc Ni - Supplementary Materials

Tobias Lojewski,[1] Mohamed F. Elhanoty,[2] Loïc Le Guyader,[3] Oscar Grånäs,[2] Naman Agarwal,[3,*] Christine Boeglin,[4] Robert Carley,[3] Andrea Castoldi,[5,6] Christian David,[7] Carsten Deiter,[3] Florian Döring,[7] Robin Y. Engel,[8] Florian Erdinger,[9,†] Hans Fangohr,[3,10,11] Carlo Fiorini,[5,6] Peter Fischer,[9] Natalia Gerasimova,[3] Rafael Gort,[3] Frank de Groot,[12] Karsten Hansen,[8] Steffen Hauf,[3] David Hickin,[3] Manuel Izquierdo,[3] Benjamin E. Van Kuiken,[3] Yaroslav Kvashnin,[2] Charles-Henri Lambert,[13] David Lomidze,[3] Stefano Maffessanti,[8] Laurent Mercadier,[3] Giuseppe Mercurio,[3] Piter S. Miedema,[8] Katharina Ollefs,[1] Matthias Pace,[4] Matteo Porro,[3,14] Javad Rezvani,[15] Benedikt Rösner,[7] Nico Rothenbach,[1] Andrey Samartsev,[3,8] Andreas Scherz,[3] Justina Schlappa,[3] Christian Stamm,[13,16] Martin Teichmann,[3] Patrik Thunstrom,[2] Monica Turcato,[3] Alexander Yaroslavtsev,[2,3] Jun Zhu,[3] Martin Beye,[8] Heiko Wende,[1] Uwe Bovensiepen,[1] Olle Eriksson,[2,17] and Andrea Eschenlohr[1,‡]

[1] *Faculty of Physics and Center for Nanointegration Duisburg-Essen (CENIDE), University of Duisburg-Essen, Lotharstr. 1, 47057 Duisburg, Germany*
[2] *Department of Physics and Astronomy, Uppsala University, 75120 Uppsala, Sweden*
[3] *European XFEL, Holzkoppel 4, 22869 Schenefeld, Germany*
[4] *Université de Strasbourg, CNRS, Institut de Physique et Chimie des Matériaux de Strasbourg, UMR 7504, 67000 Strasbourg, France*
[5] *Dipartimento di Elettronica, Informazione e Bioingegneria, Politecnico di Milano, 20133 Milano, Italy*
[6] *Istituto Nazionale di Fisica Nucleare, Sez., Milano, 20133 Milano, Italy*
[7] *Paul Scherrer Institut, Forschungsstr. 111, 5232 Villigen PSI, Switzerland*
[8] *Deutsches Elektronen Synchrotron DESY, 22607 Hamburg, Germany*
[9] *Institute for Computer Engineering, University of Heidelberg, Im Neuenheimer Feld 368, 69120 Heidelberg, Germany*
[10] *Max-Planck Institute for the Structure and Dynamics of Matter, Luruper Chaussee 149, 22761 Hamburg, Germany*
[11] *University of Southampton, Southampton SO17 1BJ, United Kingdom*
[12] *Materials Chemistry and Catalysis (MCC), Debye Institute for Nanomaterials Science, Utrecht University, Universiteitslaan 99, 3584 CG, Utrecht, The Netherlands*
[13] *Department of Materials, ETH Zurich, 8093 Zurich, Switzerland*
[14] *Department of Molecular Sciences and Nanosystems, Ca' Foscari University of Venice, 30172 Venezia, Italy*
[15] *Laboratori Nazionali di Frascati, INFN, Via Enrico Fermi 54, 00044 Frascati (Roma), Italy*
[16] *Institute for Electric Power Systems, University of Applied Sciences and Arts Northwestern Switzerland, 5210 Windisch, Switzerland*
[17] *School of Science and Technology, Örebro University, 70182 Örebro, Sweden*

(Dated: October 21, 2022)

## METHODS

In this supplementary material, we detail the steps taken in analysing the experimental data, provide further detail for the time-dependent density functional theory (TDDFT) calculations and describe the process of comparing the calculated and measured absorption spectra.

### Treatment of experimental data

In the measured absorption spectra, we find a linear background, which we attribute to the zone plate, and that leads the excited- and ground-state spectra to diverge over the energy range. We correct this background for both spectra using two linear functions with the same slope of opposite sign, thus leading the two spectra to coincide in the pre- and post-edge regions. Following the correction, the spectra are normalised so that the mean of the pre-edge region corresponds to zero, while the mean in the post-edge region corresponds to one. The measurement of the transient absorption change is then scaled with the same factor obtained from the normalisation of the spectra. This ensures continued agreement between the induced changes observed in the spectra and the evolution of the absorption changes.

### Analysing the induced changes

In order to reproduce the pumped spectrum and pump-induced change, as seen in Fig. 1(b,c) of the main paper, two modifications of the unpumped spectrum are considered, a rigid energy shift and a broadening. The energy shift is incorporated by calculating an Akima spline of the unpumped spectrum where the energy axis is shifted by ΔE. In contrast, the broadening is included via a convolution of this Akima spline with a Gaussian with

the full width at half maximum (FWHM) $\omega$. The two parameters are optimised so that the agreement of the modified Akima spline and the measured pumped spectrum is optimal in the energy range where the induced change is at its maximum (852 - 853.5 eV). By setting one of the parameters, $\omega$ or $\Delta$E, to zero, the corresponding modification is also reduced to zero, demonstrating that taking only one of these modifications into account cannot properly describe the spectral changes, as shown in Fig. 1(c) of the main paper.

For the purpose of analysing the transient absorption change at a constant $h\nu = 852.72$ eV, the response function [1] Eq. (S1) is convoluted with a Gaussian of FHWH $\omega$ and fitted to the experimental data to obtain the exponential rise $\tau_{th}$ and decay time $\tau_{e-ph}$.

$$A_0 + \Theta(t-t_0)\left(A_{th}\cdot\left[1-e^{\frac{-(t-t_0)}{\tau_{th}}}\right]\cdot\left[e^{\frac{-(t-t_0)}{\tau_{e-ph}}}\right]+ A_{e-ph}\cdot\left[1-e^{\frac{-(t-t_0)}{\tau_{e-ph}}}\right]\right) \tag{S1}$$

As the response function is obtained in the framework of the two temperature model the two time constants $\tau_{th}$ and $\tau_{e-ph}$ can be assigned to the internal thermalisation time of the electronic system and the electron-phonon coupling time respectively [1]. Following the convolution the function can be written as:

$$A_0 + e^{-z_1}\cdot(-A_{th}\cdot e^{z_2} + A_{e-ph}\cdot e^{z_1} + (A_{th}-A_{e-ph})\cdot e^{z_3} - \sqrt{\frac{1}{\omega^2}}\cdot\omega\cdot (A_{th}\cdot e^{z_1}\cdot erf\left[\frac{2t_0-t}{\omega\sqrt{2}}\right] + (A_{th}-A_{e-ph})\cdot e^{z_3}\cdot erf\left[\frac{2t_0\tau_{e-ph}+\omega^2-\tau_{e-ph}t}{\omega\tau_{e-ph}\sqrt{2}}\right] - A_{th}\cdot e^{z_2}\cdot erf\left[\frac{2t_0\tau_{e-ph}\tau_{th}+(\tau_{e-ph}+\tau_{th})\omega^2-\tau_{e-ph}\tau_{th}t}{\omega\tau_{e-ph}\tau_{th}\sqrt{2}}\right])) / 2\omega\sqrt{\frac{1}{\omega^2}} \tag{S2}$$

with:

$$z_1 = \left(\frac{1}{\tau_{e-ph}}+\frac{1}{\tau_{th}}\right)\cdot t$$
$$z_2 = \frac{(\tau_{e-ph}+\tau_{th})\cdot(4t_0\tau_{e-ph}\tau_{th}+(\tau_{e-ph}+\tau_{th})\cdot\omega^2)}{2\tau_{e-ph}^2\tau_{th}^2}$$
$$z_3 = \frac{4t_0\tau_{e-ph}+^2}{2\tau_{e-ph}^2}+\frac{t}{\tau_{th}}$$

The results are double-checked using two separate programs, one fitting the convoluted form and one where the function is convoluted during the fitting procedure leading to identical fit parameters within the error. The results of fitting the convoluted response function Eq. (S2) can be seen in Fig. 2(b) of the main paper.

## TDDFT formalism

The time-dependent Kohn-Sham (TDKS) Hamiltonian can be written as:

$$\left[\frac{1}{2}\left(-i\nabla+\frac{1}{c}\mathbf{A}_{ext}(t)\right)^2 + v_s(\mathbf{r},t) + \frac{1}{2c}\sigma\cdot\mathbf{B}_s(\mathbf{r},t) + \frac{1}{4c^2}\sigma\cdot\left(\nabla v_s(\mathbf{r},t)\times -i\nabla\right)\right]\psi_i(\mathbf{r},t) = \frac{\partial\psi_i(\mathbf{r},t)}{\partial t}, \tag{S3}$$

where c is the speed of light, $\sigma$ is the Pauli matrix, and $\mathbf{B}_s(\mathbf{r},t)$ is the effective Kohn-Sham (KS) magnetic field $\mathbf{B}_s(\mathbf{r},t) = \mathbf{B}_{ext}(t) + \mathbf{B}_{XC}(\mathbf{r},t)$, where $\mathbf{B}_{ext}(t)$ is the magnetic field of the external laser pulse and $\mathbf{B}_{XC}(\mathbf{r},t)$ is the exchange-correlation (XC) induced exchange splitting. The last term of Eq. (S3) is the spin-orbit coupling (SOC) term in its generic form, and $\psi_i(\mathbf{r},t)$ is the two component Pauli spinor. The external laser pulse is treated in the dipole approximation with a vector potential $\mathbf{A}_{\text{ext}}$(t). The atomic units (with $\hbar = e$ =m=1) are adopted in Eq. (S3).

The KS effective potential, $v_s(\mathbf{r},t)$, is a sum of three terms $v_s(\mathbf{r},t) = v_{ext}(\mathbf{r},t) + v_H(\mathbf{r},t) + v_{xc}(\mathbf{r},t)$, where $v_{ext}(\mathbf{r},t)$ is the external potential, $v_H(\mathbf{r},t)$ is the Hartree potential, and $v_{XC}(\mathbf{r},t)$ is the XC potential.

## Comparing theoretical calculations and experimental data

To directly compare the experimental and calculated absorption spectra, several steps are taken.

### *Preparing experimental data*

The experimental as well as the absorption spectra calculated from TDDFT and DFT show a varying level of contributions from excitations into the continuum. As such, these contributions have to be corrected in order to compare the data directly. In the case of the measured absorption spectra, the excitations into the continuum are corrected by subtracting a step-function of the form:

$$A_{L3}\cdot\left(\frac{1}{1+e^{\omega\cdot(E_{L3}-E)}}\right) + A_{L2}\cdot\left(\frac{1}{1+e^{\beta\omega\cdot(E_{L2}-E)}}\right) \tag{S4}$$

where $E_{L3}$ and $E_{L2}$ determine the energy position of the steps and are chosen corresponding to the maximum of

the $L_{2,3}$-edge in the ground-state spectrum. The parameter $\omega$ determines the width of the steps, and the parameter $\beta$ is added to account for the additional broadening of the $L_2$-edge due to the additional $L_2L_3V$ Coster-Kronig decay channel [2]. For the experimental spectra, the parameter $A_{L3}$ and $A_{L2}$ are set to $\frac{2}{3}$ and $\frac{1}{3}$, respectively, according to the branching ratio in nickel [3].

*Incorporation of lifetime broadening for theoretical spectra*

Furthermore, before the experimental and calculated absorption spectra can be directly compared, the calculated spectra have to be broadened to account for the lifetime broadening effects of the two absorption edges. This is done by convoluting the calculated spectra with a Lorentzian, whose FWHM increases linearly with energy, to consider the energy dependence of the Hedin-Lundqvist self-energy [4]. Here we chose to increase the FWHM of the Lorentzian by 0.1 eV for every eV on the energy scale, with the evolution of the FWHM over the energy range being shown in Fig. S1(bottom). We also consider the increased broadening of the $L_2$-edge compared to the $L_3$-edge, see above, with an increased starting value for the FWHM.

*Preparing convoluted theoretical data*

Following the convolution, a step-function Eq. (S4) is subtracted, but as the contribution of the excitations into the continuum is not identical in the calculations and the experiment, the parameters $A_{L3}$ and $A_{L2}$ have to be adjusted accordingly. Furthermore, the absolute energy scale of the theoretical calculations does not coincide with the experimentally measured one. As such, $E_{L3}$ and $E_{L2}$ are also adjusted to again correspond to the maximum of the $L_{3,2}$-edge in the ground-state spectrum. To compare the spectra, the energy scale is shifted by $\Delta$E, with the energy scale of the $L_2$-edge spectrum being shifted by the additional amount $\Delta E_{L2}$. Finally, the spectra are scaled so that the agreement between the calculated and measured ground-state spectrum is good. The parameters for the broadening are determined once in that way for the TDDFT and DFT calculations and then kept identical for all calculations in each data-set. An exemplary broadened ground state and excited spectrum is shown in Fig. S1(top) in comparison with the experimental data.

* present address: Department of Physics and Astronomy (IFA), Aarhus University, NY Munkegade 120, 8000 Aarhus C, Denmark
† present address: EXTOLL GmbH, 68159 Mannheim, Germany
‡ andrea.eschenlohr@uni-due.de

[1] N. Del Fatti, C. Voisin, M. Achermann, S. Tzortzakis, D. Christofilos, and F. Vallée, Phys. Rev. B **61**, 16956 (2000).
[2] S. Iacobucci, M. Sacchi, L. Marassi, V. Marocchi, and G. Stefani, Phys. Rev. B **59**, 9898 (1999).
[3] C. T. Chen, F. Sette, Y. Ma, and S. Modesti, Phys. Rev. B **42**, 7262 (1990).
[4] J. Mustre de Leon, J. J. Rehr, S. I. Zabinsky, and R. C. Albers, Phys. Rev. B **44**, 4146 (1991).

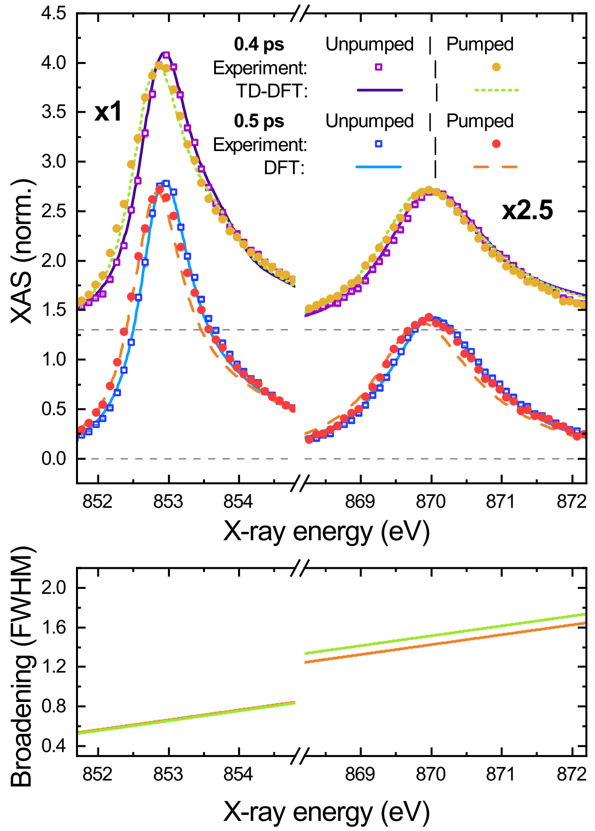


FIG. S1. (top) Ground-state (purple/blue squares) and pumped (yellow/red circles) X-ray absorption spectra at $\Delta t = 0.4$ ps and 0.5 ps, respectively, compared with the broadened calculated ground-state (purple/blue line) and excited (green dotted/red dashed line) absorption spectra obtained from TDDFT and DFT. (bottom) Evolution of the FWHM of the Lorentzian used for broadening the calculated absorption spectra from TDDFT (green) and DFT (orange) over the energy range.
